# Supplementary material for: Autonomously Untangling Long Cables
Source: arXiv:2207.07813 source file (2022-07-31)
Supplement: Supplementary file 1 [file 8-appendix.tex]

\section{Appendix}
